# Supplementary material for: Learning to Reformulate for Linear Programming
Source: arXiv:2201.06216 source file (2022-01-17)
Supplement: Supplementary file 1 [file appendix_c.tex]

\section*{Appendix B}

\subsection*{Features used in constructing biparite graph}
